# Supplementary material for: SeaPearl: A Constraint Programming Solver guided by Reinforcement Learning
Source: arXiv:2102.09193 source file (2021-04-20)
Supplement: Supplementary file 1 [file appendix.tex]

\begin{appendices}
\section{Example of an agent definition}\label{appendix:agent}

\begin{figure}[ht]
    \centering
    \begin{lstlisting}[language=Julia]
agent = RL.Agent(
    policy = RL.QBasedPolicy(
        learner = SeaPearl.CPDQNLearner(
            approximator = RL.NeuralNetworkApproximator(
                model = SeaPearl.FlexGNN(
                    graphChain = Flux.Chain(
                        GeometricFlux.GATConv(numInFeatures => 10, heads=2, concat=true),
                        GeometricFlux.GATConv(20 => 10, heads=3, concat=true),
                        GeometricFlux.GATConv(30 => 10, heads=3, concat=true),
                        GeometricFlux.GATConv(30 => 20, heads=2, concat=false),
                    ),
                    nodeChain = Flux.Chain(
                        Flux.Dense(20, 20),
                        Flux.Dense(20, 20),
                        Flux.Dense(20, 20),
                        Flux.Dense(20, 20),
                    ),
                    outputLayer = Flux.Dense(20, 30)
                ),
                optimizer = ADAM(0.0005f0)
            ),
            target_approximator = RL.NeuralNetworkApproximator(
                model = SeaPearl.FlexGNN(
                    graphChain = Flux.Chain(
                        GeometricFlux.GATConv(numInFeatures => 10, heads=2, concat=true),
                        GeometricFlux.GATConv(20 => 10, heads=3, concat=true),
                        GeometricFlux.GATConv(30 => 10, heads=3, concat=true),
                        GeometricFlux.GATConv(30 => 20, heads=2, concat=false),
                    ),
                    nodeChain = Flux.Chain(
                        Flux.Dense(20, 20),
                        Flux.Dense(20, 20),
                        Flux.Dense(20, 20),
                        Flux.Dense(20, 20),
                    ),
                    outputLayer = Flux.Dense(20, 30)
                ),
                optimizer = ADAM(0.0005f0)
            ),
            loss_func = huber_loss,
            stack_size = nothing,
            γ = 0.9999f0,
            batch_size = 1, #32,
            update_horizon = 25,
            min_replay_history = 1,
            update_freq = 10,
            target_update_freq = 200,
        ), 
        explorer = SeaPearl.CPEpsilonGreedyExplorer(
            ϵ_stable = 0.001,
            kind = :exp,
            ϵ_init = 1.0,
            warmup_steps = 0,
            decay_steps = 5000,
            step = 1,
            is_break_tie = false, 
            #is_training = true,
            seed = 33
        )
    ),
    trajectory = RL.CircularCompactSALRTSALTrajectory(
        capacity = 8000, 
        state_type = Float32, 
        state_size = state_size,
        action_type = Int,
        action_size = (),
        reward_type = Float32,
        reward_size = (),
        terminal_type = Bool,
        terminal_size = (),
        legal_actions_mask_size = (30, ),
        legal_actions_mask_type = Bool,

    ),
    role = :DEFAULT_PLAYER
)

\end{lstlisting}
    \caption{Definition of an RL agent with SeaPearl}
    \label{fig:agent_def}
\end{figure}
\end{appendices}
